# Supplementary material for: Backdoor Attacks in Peer-to-Peer Federated Learning
Source: arXiv:2301.09732 source file (2024-09-17)
Supplement: Supplementary file 1 [file appendix.tex]

% !TEX root = ../main.tex

\appendix
\textbf{Partial View Creation.} We now study the attacker's success in a more constrained setting: partial visibility. Previously, the attacker was capable of observing all of the P2PFL graph (nodes and edges). To evaluate our work in a more practical setting, now we limit this capability to a fraction of all nodes, more formally attacker can only observe $n^{*}= n \cdot o$, where $n$ is the number of total nodes, and $o$ is the observability fraction, we used $o=0.2$ in our evaluation. We constructed an observable subgraph $G'= (V', E')$ of $G= (V,E)$ with the following approach that attempts to model the lateral movement of an attacker from a single source of comprised origin. We randomly select one node $v'$ from the set $V$, and add this node to $V'$. This node  $v'$ models the single source of comprised nodes. Then, we implemented a scholastic limited depth breath first search starting at node $v$ to model lateral movement.  The limited depth part of the algorithm is trivial, the search stops when it reaches to certain depth $d$, we used $d=3$ in our experiments by reasoning of more than 3-hop lateral movement is difficult for the attacker. We modified adding a node to the rear of the queue step of the BFS algorithm, instead of immediately adding the node to the queue, we make a random experiment and based on the result of this random experiment, we add the node or not. The random experiment models whether the attacker succeeded to compromise the next host and made a lateral movement. As the random experiment, we generated a random float between 0 and 1, if the random value is less than $p^d$, we add to the node to both rear of the queue and observable nodes $V'$, where $p$ is the probability of the attacker compromising a host at depth $=1$, and $d$ is current depth. By using $p^d$, we exponentially decay the compromising probability of the attacker to make it more realistic (lateral movement becomes difficult in every hop). We used $p=0.5$ in our work. Then we constructed $E'$, by choosing the edges $e = (u,v) $ in the $E$ if both ends of the edge $u,v$ in the $V'$, or formally $E'= \{ e=(v,u) \in E \mid v, u \in V' \}$. Using $V'$ and $E'$, we created an observable subgraph $G'= (V', E')$. Then the attacker runs the PageRank algorithm on this new graph $G'$ and selects the nodes for the attack. 

\textbf{Non-iid Generation}, non-iid dataset created using Drichlet distribution for each class separately where the alpha is 10.

\begin{algorithm}[H]
\small

\KwData{Full Graph G, probability p, budget c}
%knowledge $\textsc{Agg}$}

\SetKwFunction{Diff}{Get Partial Observable SubGraph}

\SetKwData{rng}{rng}
\SetKwData{visibleBudget}{visible\_budget}
\SetKwData{visibleNodes}{visible\_nodes}
\SetKwData{queue}{queue}
\SetKwData{visitedNodes}{visited\_nodes}
\SetKwProg{Fn}{Function}{:}{}

\Fn{\Diff{$G, p, c$}}{
\BlankLine
\# create a random number generator\;
\rng $\leftarrow$ randomGenerator();

\BlankLine

\visibleBudget $\leftarrow$ numberNodes $\times$ c\;

\BlankLine
\# visible nodes\;
\visibleNodes $\leftarrow$ set()\;

\BlankLine
\# bfs queue\;
\queue $\leftarrow$ deque()\;

\BlankLine
\# bfs already visited nodes\;
\visitedNodes $\leftarrow$ set()\;

\BlankLine
\While{length(\visitedNodes) $<$ numberNodes \textbf{and} length(\visibleNodes) $<$ \visibleBudget}{
    \BlankLine
    \# choose the random node V\;
    random\_node $\leftarrow$ \choice(list(range(numberNodes)))\;

    \BlankLine
    \# random node is already visited\;
    \visitedNodes.add(random\_node)\;

    \BlankLine
    \queue.append((random\_node, 0))\;

    \BlankLine
    \# do bfs\;
    \While{length(\queue) $>$ 0}{
        \BlankLine
        \# pop the curr node with its depth from queue\;
        node, node\_depth $\leftarrow$ \queue.popleft()\;

        \BlankLine
        \# neighbours of node\;
        adjs $\leftarrow$ nx.neighbors(graph, node)\;

        \BlankLine
        \# traverse node's neighbors\;
        \ForEach{adj \textbf{in} adjs}{
            \BlankLine
            \# if adj already visited, ignore\;
            \If{adj \textbf{in} \visitedNodes}{
                \textbf{continue}\;
            }

            \BlankLine
            \# if depth is more than maximum, ignore\;
            \If{node\_depth + 1 $>$ d}{
                \textbf{continue}\;
            }

            \BlankLine
            \# generate a random value between 0 and 1\;
            random\_val $\leftarrow$ \rng.random()\;

            \BlankLine
            \# level visibility threshold, p\textasciicircum(d+1)\;
            threshold $\leftarrow$ p\textasciicircum(node\_depth + 1)\;

            \BlankLine
            \If{random\_val $\leq$ threshold \textbf{and} length(\visibleNodes) $<$ \visibleBudget}{
                \visibleNodes.add(adj)\;
                \queue.append((adj, node\_depth + 1))\;
            }

            \BlankLine
            \visitedNodes.add(adj)\;
        }
    }
}

\BlankLine
 \visibleNodes $\leftarrow$ list(\visibleNodes)\;
return \visibleNodes \;
}

\caption{Generation of Partial Observable subgraph $G'$}
\label{alg:partialObservability}
\end{algorithm}
